# Supplementary material for: Smartphones with UWB: Evaluating the Accuracy and Reliability of UWB Ranging
Source: arXiv:2303.11220 source file (2023-03-20)
Supplement: Supplementary file 1 [file appendix.tex]

% !TeX root = ../main.tex

\section*{Appendix}

\begin{figure}[!t]
    \centering 
    \scalebox{0.9}{\input{figures/eval/devices/polar_plots/polar_0_Outside_5.pgf}}
    \caption{\textbf{Outside measurements at \SI{5}{\metre} distance.} One full base rotation $\theta$ of \ac{gwen} and arm rotation at $\phi=\SI{0}{\degree}$. Fewer measurements failed, but the overall error increased compared to an arm rotation of $\phi=\SI{90}{\degree}$.}\label{fig:outdoor_polar_0_arm}
\end{figure}
